# Supplementary material for: Safe Deep Reinforcement Learning by Verifying Task-Level Properties
Source: arXiv:2302.10030 source file (2023-02-20)
Supplement: Supplementary file 1 [file supplemental.tex]

\section*{Appendix: Results in Terminal Environments}
The two rows of Figure \ref{fig:suppl_exp_results_T} show the evaluation in the (T) tasks. 
In \textit{Fixed\_obs\_T}, PPO achieves the highest success and cost, while safety-informed PPO methods (LPPO, PPO\_\{cost, violation\}) share similar successes. Penalty-based implementations (PPO\_\{cost, violation\}) also reduce the cost and violation, while LPPO fails at maintaining the threshold set to 0.45. The value-based implementations achieve similar results, slightly improving the average violations in the penalty-based versions. The \textit{Dynamic\_obs\_T} has different violation results. The violation-based methods achieve the lowest number of violations through training. In more detail, the $\approx0.2\%$ and $\approx0.7\%$ improvement of \{DuelDDQN, PPO\}\_violation over the cost counterparts at convergence maps to 120 and 420 fewer states where the policy chooses an action that leads to a collision. Even when violations rarely occur (i.e., one per episode), the information carried by the violation nearby unsafe states results in a significant advantage, maintaining similar or higher successes over non-violation-based approaches.

\begin{figure*}[h]
    \centering
    \includegraphics[width=\textwidth]{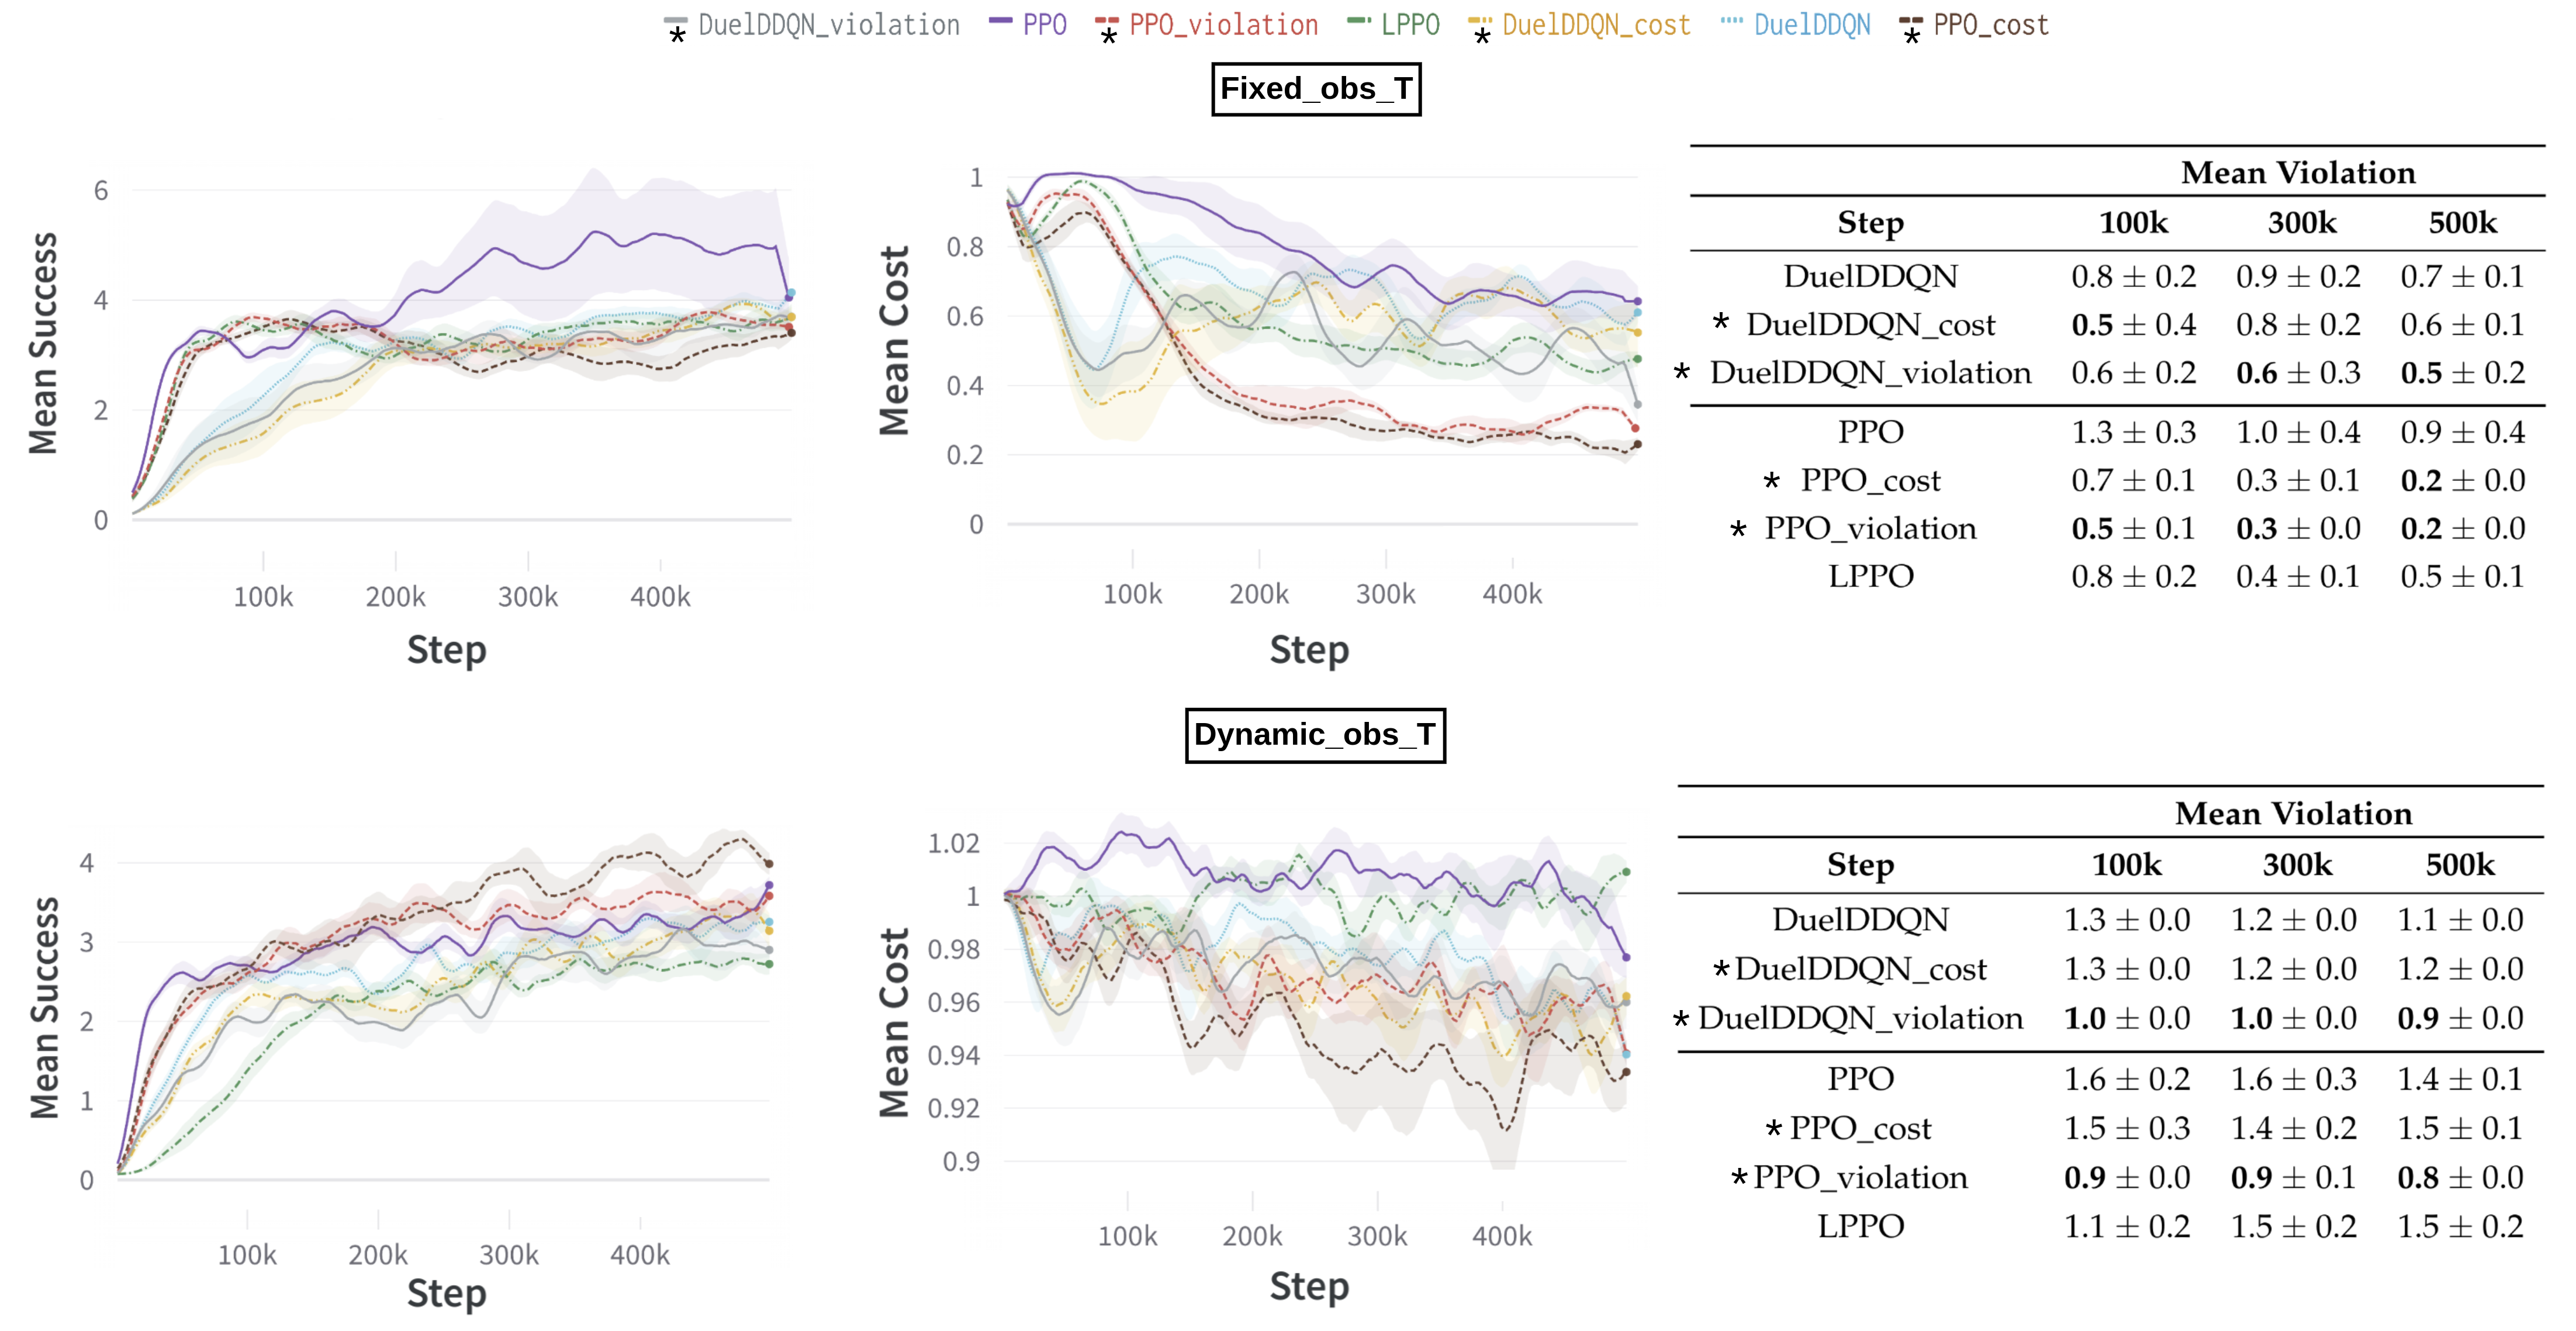}
    \caption{The two rows show average success, cost, and violation in the (T) environments for DuelDDQN, PPO, the cost and violation penalty versions, and LPPO.}
    \label{fig:suppl_exp_results_T}
\end{figure*}

Table \ref{tab:suppl_verification_T} shows the average formal violation value computed on the models at convergence in the terminal environments. Crucially, algorithms trained with our approximate violation value achieve a lower violation, which translates into a lower number of collisions.

\begin{table*}[h]
\centering
    \caption{Average formal violation for the models at convergence in T environment. Our violation-based penalty algorithm is the safest overall, as a lower violation value translates into fewer collisions.}
    \label{tab:suppl_verification_T}
    \includegraphics[width=0.8\linewidth]{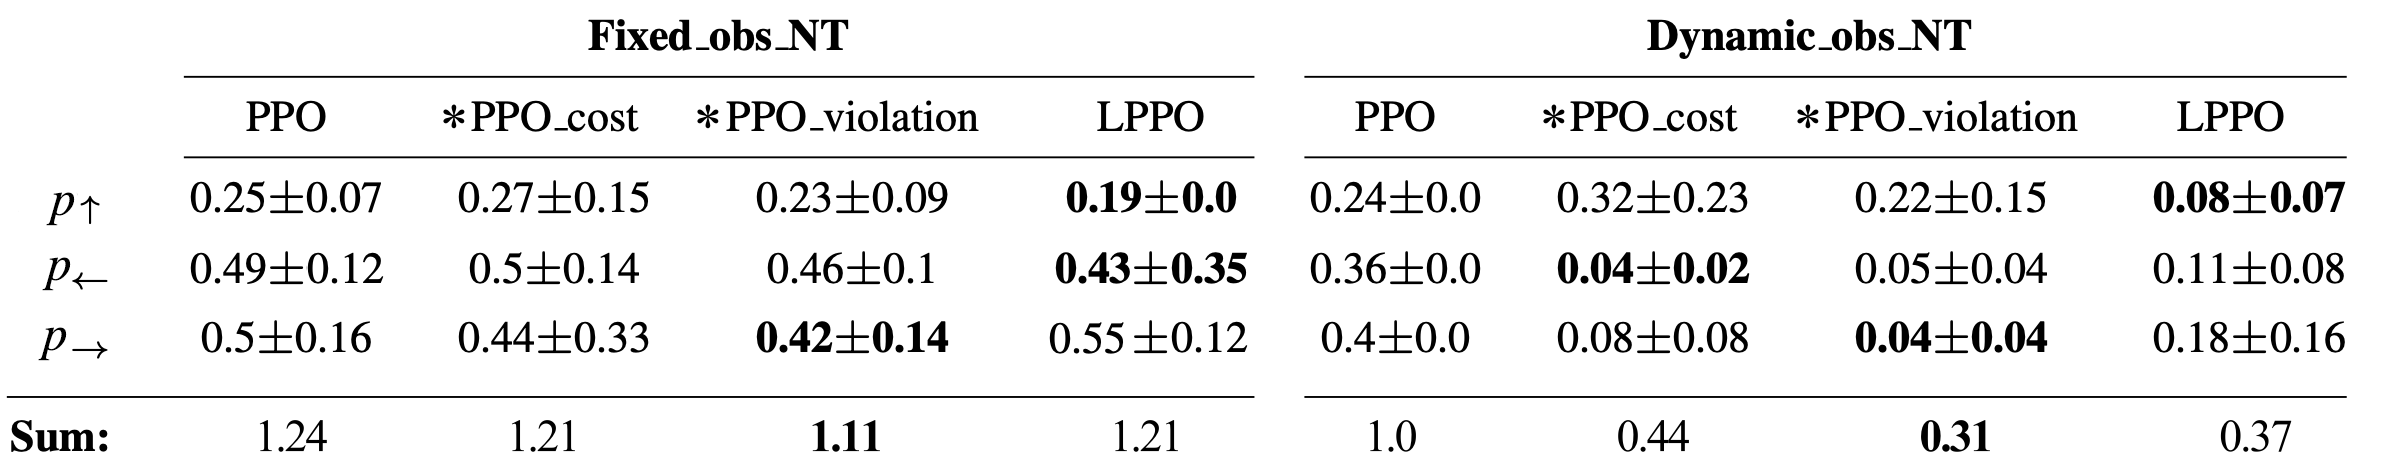}
\end{table*}

\begin{figure*}[h!]
    \centering
    \includegraphics[width=\linewidth]{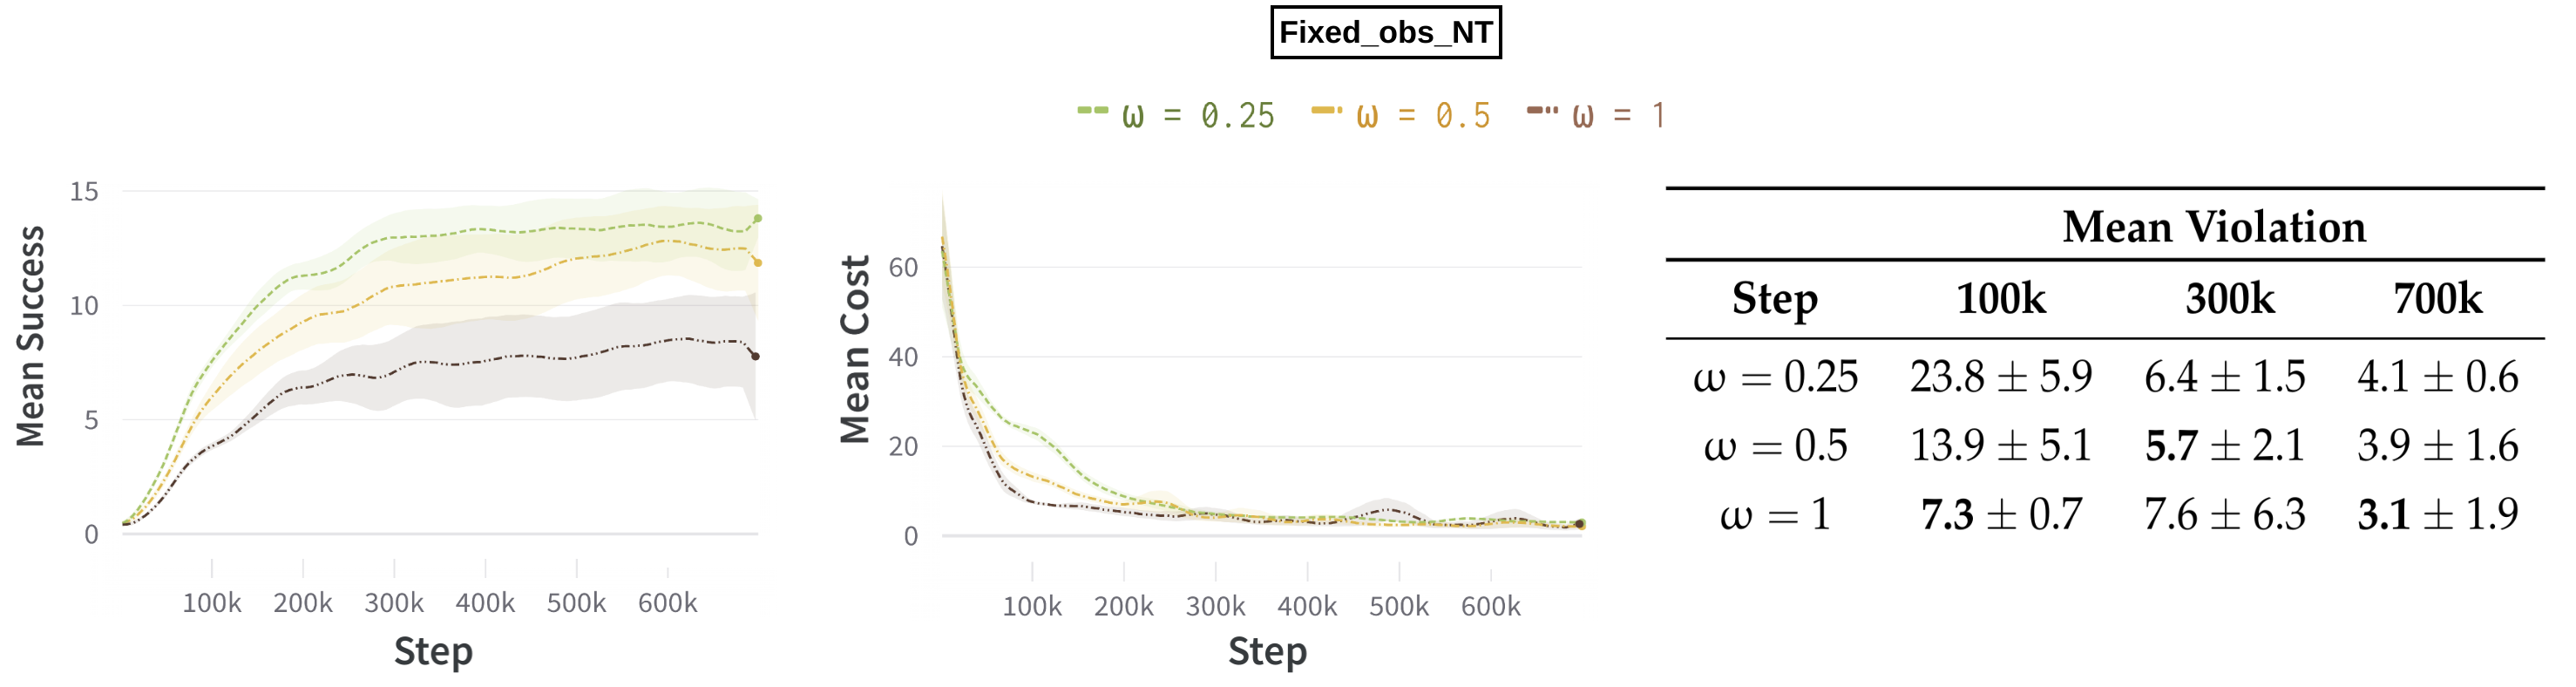}
    \caption{Effects of $\omega$ on PPO\_cost. Values $< 1$ give more importance to the reward, resulting in more unsafe behaviors.}
    \label{fig:suppl_omega}
\end{figure*}

\section*{Appendix: Impact of penalty regularization}
Figure \ref{fig:suppl_omega} shows additional experiments on \textit{Fixed\_obs\_NT} to investigate the effects of a penalty regularization term, $\omega$. In particular, we found a good trade-off between performance and safety with $\omega = 1$, while lower values penalize the reward, leading to more risky behaviors.

\section*{Appendix: Hyper-parameters}
We performed an initial grid search among common hyper-parameters from prior work \cite{PPO, DuelDDQN, SafetyGym, AAAI_Sos}. This evaluation led us to use the same DNN architecture for all the algorithms in the environments but higher total steps in more complex tasks to achieve reasonable navigation performance. In more detail, we use a 2-ReLU layer MLP with 64 hidden units each to model actors and critics. Moreover, Table \ref{tab:hyperparameters} shows a detailed overview of the other main parameters used among the considered algorithms. Note that missing parameters are shared with the baseline algorithm (e.g., LPPO parameters are the same as PPO).

\begin{table*}[h!]
\centering
\caption{Detailed overview of the considered hyper-parameters.}
\label{tab:hyperparameters}
\begin{tabular}{llr}
\toprule
\textbf{Environment Steps}     & Fixed\_obs\_T              & 500k                 \\
                               & Dynamic\_obs\_T            & 500k                 \\
                               & Fixed\_obs\_NT             & 700k                 \\
                               & Dynamic\_obs\_NT           & 2M                   \\
                               & steps per episode          & 500                  \\ \midrule
\textbf{Penalties}             
& $\beta$ & 0.0005 \\
& cost                       & 1                    \\
                               & violation                  & Computed                           \\ \midrule
\textbf{Approximate Violation} & $\epsilon$    & 0.05                 \\
                               & points per property        & 10000                \\ \midrule
\textbf{DuelDDQN SaAgents}       & $\gamma$      & 0.99                 \\
                               & $\tau$        & 0.05                 \\
                               & buffer capacity            & 10000                \\
                               & batch size                 & 64                   \\ \midrule
\textbf{PPO Agents}            & $\gamma$      & 0.9                  \\
                               & clip                       & 0.2                  \\
                               & GAE $\lambda$ & 0.97                 \\
                               & update epochs              & 10                   \\
                               & update frequency           & 5                    \\ \midrule
\textbf{LPPO Agents}           & multiplier                 & 1.0                  \\
                               & cost thresholds             & Fixed\_obs\_T: 0.48   \\
                               &                            & Dynamic\_obs\_T: 0.98 \\
                               &                            & Fixed\_obs\_NT: 4.5   \\
                               &                            & Dynamic\_obs\_NT: 11  \\ \bottomrule
\end{tabular}
\end{table*}
